# Supplementary material for: Exploring Defeasibility in Causal Reasoning
Source: arXiv:2401.03183 source file (2024-06-27)
Supplement: Supplementary file 1 [file metrics.tex]

In this section, we describe the details of another causal strength metric proposed by us: CTCW. We first introduce its motivation and definition in Appendix~\ref{appendix:ctcw:motivation}. Then we show the experimental results of CTCW in Appendix~\ref{appendix:ctcw:results}, including the results on capturing the causal strength changes brought by supporters and defeaters in \shorttitle. Moreover, we also discuss the formulation of concatenation rules we used for CTCW in Appendix~\ref{appendix:ctcw:concatenation}. Appendix~\ref{appendix:ctcw:case} is a case study to verify the effectiveness of CTCW. 
We thoroughly discuss the issues and flaws of CTCW in Appendix~\ref{appendix:ctcw:issues} and \ref{appendix:ctcw:sumnot1}. We present several promising topics related to causal strength in Appendix~\ref{appendix:ctcw:discussion}.

\subsection{Motivation and Definition of CTCW} \label{appendix:ctcw:motivation}
\noindent\textbf{Motivation.\tbfspace}In practice, temporal and causal words provide important hints for a causal relationship. Causal words like ``because'' and ``therefore'' provide useful indicators for a causal relationship. For instance, ``A happens because B happens'' represents that B causes the occurrence of A. Similarly, patterns like ``A happens therefore B happens'' represent that A causes the occurrence of B. In the same manner, temporal indicators such as ``before'' and ``after'' furnish essential chronological context for understanding causal relationships, given that the cause invariably precedes the effect. For example, statements constructed in the pattern ``A occurs after B'' imply that B may serve as the causal agent for A. Likewise, statements constructed in the pattern ``A occurs before B'' imply that A may serve as the causal agent for B.

\noindent\textbf{Definition of CTCW.\tbfspace} With the inspiration above, we define the causal strength between $C$ and $E$ as: 
\begin{equation}
    \causalstrength{C}{E} = \sum_{w \in M^{+}} p(w) - \sum_{w \in M^{-}} p(w). 
\end{equation}
where $M^{+} = \{\text{before, therefore}\}$ and $M^{-} = \{\text{after, because}\}$. Specifically, $M^{+}$ is the set of causal and temporal tokens that support a causal relationship between $C$ and $E$. Effectively, $C$ leads to the occurrence of $E$. On the other hand, $M^{-}$ is the set of causal and temporal tokens that support the causal relationship where $E$ leads to the occurrence of $C$. Lastly, \( p(w) \) represents the probability that a specific token \( w \) is selected from $M^{+}$ and $M^{-}$ to replace the masked position according to a large language model such as ChatGPT when presented with the contextual input \( C + \text{[MASK]} + E \). This formula conceptualizes the idea that a causal relationship is provided by the hints of temporal and causal cues, and the extent of the causal strength is given by the probability of these temporal and causal words given by large language models like ChatGPT. 
The prompt we give to the ChatGPT is described in more detail in Appendix~\ref{appendix:ctcw:case}. 

\subsection{Experimental Results on CTCW} \label{appendix:ctcw:results}
\noindent\textbf{Experimental Results on \shorttitle in Capturing Causal Strength Changes Brought By Supporters and Defeaters.\tbfspace} The experimental results on \shorttitle are shown in Table~\ref{tab:appendix:templates}. From the results, we can observe that CTCW exhibits notable performance on both supporters and defeaters: it achieves an accuracy of 77.2\% on supporters and 86.6\% on defeaters with appropriate prompt templates. 
Here the accuracy is calculated in the same way as that in the caption of Table~\ref{tab:causal_metrics} in \S~\ref{sec:discussions:challenges}. 
In contrast to ROCK and CEQ, which achieve an average accuracy of only 50\%, the CTCW algorithm demonstrates a significant improvement with an average accuracy of 81.9\%. However, CTCW is influenced greatly by the prompts given to ChatGPT. Besides, it remains a black box for users and lacks explainability, which is less attractive compared with the CESAR metric in \S~\ref{sec:causal_strength}.  

\noindent\textbf{Shift of Causal Strength Given by CTCW With the Incorporation of Supporters and Defeaters.\tbfspace} \label{appendix:metrics:shift}
We also plot the overall shift of the CTCW values with the incorporation of supporters and defeaters in Figure~\ref{fig:appendix:shift_ctcw}. We observe that with the incorporation of supporters, the distribution of CTCW shifts right, which means that the presence of supporters increases the causal strength between the cause and effect. Besides, we find that the presence of defeaters shifts the distribution of CTCW value to the left side, which means that defeaters significantly decrease the causal strength between cause and effect. From the results, we can safely conclude that CTCW precisely captures the characteristics of causal strength. CTCW proves itself to be a satisfying metric for capturing the causal strength changes brought by supplementary information. 
\begin{figure}[htp!]
    \centering
    \includegraphics[width=0.52\textwidth]{defeasible_reasoning/figures/causal_strength_shift_ctcw.pdf}
    \caption{The shift of causal strength value given by CTCW with the incorporation of supporters and defeaters. We plot the distribution of the causal strength using kernel density estimate~(KDE), which could represent the data distribution in a continuous probability density curve.}
    \label{fig:appendix:shift_ctcw}
\end{figure}

\subsection{Discussion of Formulations of Concatenation Rules in CTCW}
\label{appendix:ctcw:concatenation}
As we have to look into details about how the causal strength changes with the \textbf{incorporation} of supporters or defeaters, it is important to design different concatenation rules to accurately reflect the operation of incorporation. We design three types of concatenation rules and describe them in detail in the following text. 

\subsubsection{Different Concatenation Rules} 
\noindent\textbf{Concatenation Rule with \textit{``and''}.\tbfspace} A straightforward template for concatenation is to use the word \textit{and} for concatenation. Namely, the concatenation operation $\oplus$ is defined as:  
\begin{equation}
    C \oplus A/D = C + [\text{and}] + A/D. 
\end{equation}
However, we identified that in some cases the resulting phrases are semantically or grammatically incorrect, which poses significant challenges for large-scale language models. Several cases are present as follows: 
\begin{enumerate}
    \item \textit{Tim mentions in a speech that he is sick of the oligarchy in his country and Tim is still sick of the oligarchy [MASK] Tim is killed for causing people to think freely.} Adding the supporter according to the general template just creates redundancy and confuses the LLM, lowering the probability of replacing the mask with some meaningful casualty indication token.  
    \item \textit{Bill wasn't wearing a helmet when he fell off his motorcycle and Bill hits his head [MASK] Bill was still suffering from brain damage.} Here we have an example where the supporter sentence is grammatically inconsistent with the other sentences (the supporter sentence is written in the present tense while the other parts are given in the past tense), making the whole statement grammatically incorrect and creating temporal ambiguity. 
\end{enumerate}
From these examples, we could safely conclude that the general template  \textit{``and''} is not appropriate for all cases. 

\noindent\textbf{Concatenation Rule with \textit{``it is a fact that''}.\tbfspace} 
We observe that in most cases supporters signify general knowledge facts or confirmation statements. Motivated by this observation, we devise the following template for the concatenation of cause and supporter/defeater: 
\begin{equation}
    C \oplus A/D = \text{It is the fact that} + A/D. \,\text{{So,}} + C 
\end{equation}
Now the above examples turn into: 
\begin{enumerate}
    \item ID 7543: \textit{It is the fact that Tim is still sick of the oligarchy. So, Tim mentions in a speech that he is sick of the oligarchy in his country [MASK] Tim is killed for causing people to think freely.}
    \item ID 9789: \textit{It is the fact that Bill hits his head. So, Bill wasn't wearing a helmet when he fell off his motorcycle [MASK] Bill was still suffering from brain damage.}
\end{enumerate}

\noindent\textbf{Concatenation Rule with \textit{``and later''}.\tbfspace} 
To emphasize the temporal relationship between cause and supporter/defeater, we design a new concatenation rule for supporter/defeater: 
\begin{equation}
    C \oplus A/D = C + [\text{and later}] + A/D.
\end{equation}

\subsubsection{Results of Different Concatenation Rules in Capturing Causal Strength Changes Brought by Supporters and Defeaters}
We list the results of these three investigated metrics on causal strength in Table~\ref{tab:appendix:templates}. From the results, we can conclude that for supporters, the concatenation template ``it is fact that'' works the best and achieves an accuracy of 77.2\%. For defeaters, the concatenation template ``and later'' works the best and achieves an accuracy of 86.6\%. Generally speaking, the concatenation template ``it is fact that'' achieves a good balance between capturing the causal strength changes brought by supporters and defeaters. 

\begin{table}[htp!]
    \centering
    \resizebox{0.35\textwidth}{!}{
    \begin{tabular}[c]{lll}
        \toprule 
        Template & Supporter & Defeater \\
        \midrule
        \textit{and} & 59.4 & 75.0 \\
        \textit{it is fact that} & \textbf{77.2} & 61.8 \\
        \textit{and later} & 37.4 & \textbf{86.6} \\
        % \textit{Combined template} & 77.2 & 86.6 \\
        \bottomrule
   \end{tabular}
   }
    \caption{Performance of our causal metric for each template we propose. Accuracy is computed as follows: If the causal strength of two events supplemented with a supporter does not decrease compared to the case when no supplementary information is given, we count that as a correct result. If the causal strength of two events supplemented with a defeater does not increase compared to the case when no supplementary information is given, we count that as a correct result. }
    \label{tab:appendix:templates}
\end{table}

\subsection{Case Study} \label{appendix:ctcw:case}
To better present how we use CTCW in our experiments, we present a case study on CTCW. 
For the following studying cases, we use \texttt{gpt-3.5-turbo}  as the model to do the prompt. Besides, the input prompt consists of two parts, the first part is the input text while the second part is the detailed instruction we give to the model.  

\subsubsection{Causal Strength Between Cause and Effect} \label{appendix:ctcw:case:ce}
For the causal strength between cause and effect, the prompt given to ChatGPT is as follows: 
 \begin{center}
\mybox[gray!20]{
C = ``The earthquake hit a city.'' \\
E = ``Mental health issues arose.'' \\
``The earthquake hit a city [MASK] mental health issues arose.'' \vspace{1em} \\
``Give the probabilities for each of the listed words to replace the [MASK]:\\
- after\\
- before\\
- therefore\\
- because\\
such that, \\
- "after" implies that A happened later than B\\
- "before" implies that A happened earlier than B\\
- "therefore" implies that A causes B, i.e., A is the cause of B, and B is the effect of A\\
- "because" implies that B causes A, i.e., A is the effect of B, and B is the cause. \\
Keep in mind that "therefore" and "because" have opposite meanings in this context.
The sum of probabilities should not exceed 1.0, but if words don't fit well enough, the sum can be less than 1.0. The probabilities should be based on the descriptions above. If a word does not fit well, it should have zero probability. The cause should always precede the effect. Try to list only probabilities without further explanations.''
}
\end{center}

The results that the gpt-3.5-turbo model yields for this example are the following: 
\begin{table}[htp!]
    \centering  
    \begin{tabular}[c]{lc}
        \toprule 
        Word & Probability of word  \\
        \midrule
        \textit{after} & 0.30  \\
        \textit{before} & 0.50  \\
        \textit{therefore} & 0.20  \\
        \textit{because} & 0.00  \\
        \bottomrule
   \end{tabular}
    \caption{Probability of contrastive temporal and causal words on cause and effect given by ChatGPT.}
    \label{tab:appendix:templates_1}
\end{table}

Based on the CTCW metric, the causal strength is: 
\begin{equation*}
\begin{split}
    \causalstrength{C}{E} &= \sum_{w \in M^{+}} p(w) - \sum_{w \in M^{-}} p(w) \\ 
    &= 0.50 + 0.20 - 0.30 - 0.00 \\
    &= 0.40
\end{split}.
\end{equation*}

\subsubsection{Causal Strength Between Cause-Supporter and Effect} \label{appendix:ctcw:case:cse}
With the incorporation of supporters, now the prompt given to ChatGPT becomes: 
\begin{center}
\mybox[gray!20]{
    C = ``The earthquake hit a city.'' \\
    E = ``Mental health issues arose.''\\
    A = ``A disaster usually leads to suffering and loss of people'' \\
    ``It is a fact that a disaster usually leads to suffering and loss of people. So, the earthquake hit a city [MASK] mental health issues arose.'' \vspace{1em}
    \\ 
    ``Give the probabilities for each of the listed words to replace the [MASK]:\\
- after\\
- before\\
- therefore\\
- because\\
such that, \\
- "after" implies that A happened later than B\\
- "before" implies that A happened earlier than B\\
- "therefore" implies that A causes B, i.e., A is the cause of B, and B is the effect of A\\
- "because" implies that B causes A, i.e., A is the effect of B, and B is the cause. \\
Keep in mind that "therefore" and "because" have opposite meanings in this context.
The sum of probabilities should not exceed 1.0, but if words don't fit well enough, the sum can be less than 1.0. The probabilities should be based on the descriptions above. If a word does not fit well, it should have zero probability. The cause should always precede the effect. Try to list only probabilities without further explanations.''
}
\end{center}

The results that the gpt-3.5-turbo model yields for this concatenation of supporters are the following: 
\begin{table}[htp!]
    \centering  
    \begin{tabular}[c]{lc}
        \toprule 
        Word & Probability of word  \\
        \midrule
        \textit{after} & 0.20  \\
        \textit{before} & 0.10  \\
        \textit{therefore} & 0.70  \\
        \textit{because} & 0.00  \\
        \bottomrule
   \end{tabular}
    \caption{Probability of contrastive temporal and causal words on cause with supporter and effect given by ChatGPT. }
    \label{tab:appendix:templates_2}
\end{table}

Based on the CTCW metric, the causal strength now turns into: 
\begin{equation*}
\begin{split}
    \causalstrength{C}{E} &= \sum_{w \in M^{+}} p(w) - \sum_{w \in M^{-}} p(w) \\ 
    &= 0.10 + 0.70 - 0.20 - 0.00 \\
    &= 0.60
\end{split}.
\end{equation*}
Compared with the causal strength on cause and effect, the CTCW value changes from 0.40 to 0.60. It shows the supporter increases the cause strength betwen cause and effect, which agrees well with human intuition. 

\subsubsection{Causal Strength Between Cause-Defeater and Effect } \label{appendix:ctcw:case:cde}
With the incorporation of defeaters, now the prompt given to ChatGPT turns into: 
\begin{center}
    \mybox[gray!20]{
    C = ``The earthquake hit a city.'' \\
    E = ``Mental health issues arose.''\\
    D = ``Lots of mental health assistance is provided.'' \\
    ``The earthquake hit a city, and later lots of mental health assistance was provided [MASK] mental health issues arose.'' \vspace{1em} \\
    ``Give the probabilities for each of the listed words to replace the [MASK]:\\
- after\\
- before\\
- therefore\\
- because\\
such that, \\
- "after" implies that A happened later than B\\
- "before" implies that A happened earlier than B\\
- "therefore" implies that A causes B, i.e., A is the cause of B, and B is the effect of A\\
- "because" implies that B causes A, i.e., A is the effect of B, and B is the cause. \\
Keep in mind that "therefore" and "because" have opposite meanings in this context.
The sum of probabilities should not exceed 1.0, but if words don't fit well enough, the sum can be less than 1.0. The probabilities should be based on the descriptions above. If a word does not fit well, it should have zero probability. The cause should always precede the effect. Try to list only probabilities without further explanations.''
}
\end{center}

The results that the gpt-3.5-turbo model yields for this concatenation of defeaters are the following: 
\begin{table}[htp!]
    \centering  
    \begin{tabular}[c]{lc}
        \toprule 
        Word & Probability of word  \\
        \midrule
        \textit{after} & 0.30  \\
        \textit{before} & 0.10  \\
        \textit{therefore} & 0.40  \\
        \textit{because} & 0.00  \\
        \bottomrule
   \end{tabular}
    \caption{Probability of words given by ChatGPT. }
    \label{tab:appendix:templates_3}
\end{table}

Based on the CTCW metric, the causal strength now turns into: 
\begin{equation*}
\begin{split}
    \causalstrength{C}{E} &= \sum_{w \in M^{+}} p(w) - \sum_{w \in M^{-}} p(w) \\ 
    &= 0.10 + 0.40 - 0.30 - 0.00 \\
    &= 0.20
\end{split}.
\end{equation*}
Compared with the causal strength on cause and effect, the CTCW value changes from 0.40 to 0.20. It shows that the causal strength between cause and effect decreases with the incorporation of the defeater event, which agrees well with human intuition.

\subsection{Issues with CTCW} \label{appendix:ctcw:issues}
``There are spots even on the Sun.'' It is worthwhile to highlight several limitations of the proposed CTCW metric: 
(i) The sets for positive temporal causal words and negative temporal causal words are relatively small, which may be insufficient to capture all of the necessary temporal and causal information; 
(ii) We found in the experiment that the values given by ChatGPT have some degree of fluctuation, which is inherent in the stochastic nature of large-scale language models like ChatGPT. 
(iii) Sometimes the total probability given by ChatGPT is over 1.0 even though it is instructed to not be over 1.0. We find in Figure~\ref{fig:appendix:shift_ctcw} that a small portion of causal strength is over 1.0 or less than -1.0. This is further discussed in Appendix~\ref{appendix:ctcw:sumnot1}. 

\subsection{Discussion of the Situation That the Sum of Probability Returned by ChatGPT Is Not 1}
\label{appendix:ctcw:sumnot1}
The instruction given to ChatGPT states: ``The sum of probabilities should not exceed 1.0, but if words don't fit well enough, the sum can be less than 1.0.'' This guideline tries to ensure that the probability value remains capped at 1. It's important to note that we don't mandate the combined probabilities of temporal and causal terms in our predefined set to be exactly 1. This stipulation arises from the inherent challenges of comprehensively capturing all possible temporal and causal terms in our vocabulary set. In fact, achieving complete inclusivity of such terms is either highly difficult or practically infeasible. Overloading the prompt for ChatGPT with an excessive number of temporal and causal terms risks introducing confusion to the model's output.

The focus of CTCW primarily centers on two principles:
\begin{itemize}
    \item The causal difference implied by the contrasting temporal words, i.e., \textit{before} and \textit{after}, and the contrasting causal words \textit{because} and \textit{therefore}.
    \item The dissimilarity between these contrasting terms denotes the underlying causal and temporal relationship between two events. 
\end{itemize}
Through this approach based on contrastive temporal and causal words, we prompt language models like ChatGPT to indirectly measure the causal strength between two events. It paves a new way to utilize LLMs to quantitatively measure the causal strength between two events. 

\subsection{More Discussion on Causal Strength Evaluation} \label{appendix:ctcw:discussion}
CTCW sheds light on how to use contrastive temporal and causal words to calculate the value of causal strength. However, due to the limit and dependence on ChatGPT, it also poses some challenges such as fluctuations. There are several interesting and promising topics related to causal strength evaluation that are worth investigating: 
\begin{itemize}
    \item Fine-grained causal strength evaluation between words or phases: for language, the causal relationship is gathered between certain words or phase pairs. For instance, ``exercise'' and ``health'' have higher word-to-word causal strength. The CESAR metric provided in \S~\ref{sec:causal_strength} is one of this line of work. 
    \item Explainability of causal strength: instead of only predicting the causal strength, the detailed explanation of why the model gives this prediction helps us better understand the logic behind the causality. For instance, the reason that the model gives the higher causal strength value between ``exercise regularly'' and ``lose weight'' is that ``exercise can increase one's metabolism and thus burn calories, the burn of calories will get rid of the fat''. 
    \item Adaption to new changes: in domains like law and finance, the causal relationship changes with the changes in laws and regulations. It is important to capture and reflect the changes. 
\end{itemize}

\begin{figure*}
    \centering
    \includegraphics[width=1.0\textwidth]{defeasible_reasoning/figures/long_term_effect_without_keyword_grey.png}
    \caption{Cause-effect pair collection without hints of keywords. }
    \label{fig:appendix:long_term_effect_without_keyword}
\end{figure*}

\begin{figure*}
    \centering
    \includegraphics[width=1.0\textwidth]{defeasible_reasoning/figures/long_term_effect_with_keyword_grey.png}
    \caption{Cause-effect pair collection with hints of keywords. }
    \label{fig:appendix:long_term_effect_with_keyword}
\end{figure*}

\begin{figure*}
\centering
\begin{minipage}{.5\textwidth}
  \centering
  \includegraphics[width=.95\linewidth]{defeasible_reasoning/figures/defeasibility_grey.png}
  \vspace{4em}
  \captionof{figure}{Collection of defeasibility~(supporters and defeaters).}
  \label{fig:appendix:defeasibility}
\end{minipage}
\end{figure*}

\begin{figure*}
    \centering
    \includegraphics[width=0.9\textwidth]{defeasible_reasoning/figures/long_term_effect_refinement_grey.png}
    \caption{Refinement of causality.}
    \label{fig:appendix:refinement_causality}
\end{figure*}

\begin{figure*}
    \centering
    \includegraphics[width=0.9\textwidth]{defeasible_reasoning/figures/assumption_refinement_grey.png}
    \caption{Refinement of supporters. }
    \label{fig:appendix:assumption_refinement}
\end{figure*}

\begin{figure*}
    \centering
    \includegraphics[width=0.9\textwidth]{defeasible_reasoning/figures/defeater_refinement_grey.png}
    \caption{Refinement of defeaters. }
    \label{fig:appendix:defeater_refinement}
\end{figure*}
