# Supplementary material for: Exploring Defeasibility in Causal Reasoning
Source: arXiv:2401.03183 source file (2024-06-27)
Supplement: Supplementary file 2 [file turk.tex]

In this section, we present the interfaces we use in Amazon Mechanical Turk for annotation and refinement of \shorttitle. 

\noindent\textbf{Interface for Annotation of Cause-Effect Pairs.\tbfspace}  
Figure~\ref{fig:appendix:long_term_effect_without_keyword} and Figure~\ref{fig:appendix:long_term_effect_with_keyword} show the interface for annotations of cause-effect pairs without and with keywords respectively. Apart from the typical examples we give to better guide the annotation of cause-effect pairs, we also give the domain label to the annotators to help them write in-domain annotations. Specifically, we give different time intervals for them to decide on the interval between cause and effect. The difference between the collection of cause-effect pairs with and without keywords is that we give the keywords of a certain domain to help annotators write keyword-related cases. The collection of \shorttitle is under the participation agreement and acceptable use policy of Amazon Mechanical Turk. 

\noindent\textbf{Interface for Annotation of Defeaters and Supporters. \tbfspace}  
The interface for the annotation of defeaters and supporters is shown in Figure~\ref{fig:appendix:defeasibility}. We first give several typical cases about supporters and defeaters and then provide the cause and its effect for their annotations. Notice that we ask the same annotators to write both supporter and defeater, which increases the complementation between supporter and defeater. The reason why we explicitly ask them to write the supporter and defeater is that the supporter and defeaters are more related and can help each other. 

\noindent\textbf{Interface for Refinement of Cause-Effect Pairs. \tbfspace}
The interface for the refinement of cause-effect pairs is shown in Figure~\ref{fig:appendix:refinement_causality}. Besides typical correct and wrong examples of causality, each assignment consists of two cause-effect pairs, one of which is the annotation that needs judgment while the other is a golden example that we know is valid or invalid. These golden examples are carefully written by us and we make sure that they can be classified without confusion. In this way, we further filter the assignments that are randomly or cursorily annotated. Though this way causes additional costs, it ensures the high quality of our final collected dataset.  

\noindent\textbf{Interface for Refinement of Supporters and Defeaters. \tbfspace}
The interfaces for the refinement of supporters and defeaters are shown in Figure~\ref{fig:appendix:assumption_refinement} and Figure~\ref{fig:appendix:defeater_refinement} respectively. Similarly, each assignment consists of two cause-effect-supporter or cause-effect-defeater triples, one of which is the annotation that needs judgment while the other is a golden example that we know is valid or invalid. For the supporter, we ask them to give their judgment based on whether the given supporter supports or makes the causality between the cause and the effect stronger. For the defeaters, we ask them to give their judgment based on whether the given defeater can overthrow or weaken the causality between the cause and the effect.
